# Supplementary material for: Anti-noise window: Subjective perception of active noise reduction and effect of informational masking
Source: arXiv:2307.05533 source file (2023-07-08)
Supplement: Supplementary file 3 [file next-appendix.tex]

\setcounter{table}{1}
